# Supplementary material for: Streaming Detection of Queried Event Start
Source: arXiv:2412.03567 source file (2024-12-04)
Supplement: Supplementary file 3 [file zs_clip.tex]

python meassure_latency.py --mode predict --task_name sdqes --classification_layer_name cosine_similarity --data_path /vision/u/eatang/sdas/ --video_path /scr/ego4d_full_frames/ --backbone_name clip_ViT-B/16 --seed 42 --num_workers 0 --gpus 1 --batch_size 8 --n_frames 60 --frame_sample_rate 1 --temporal_pooling_name identity --criterion_name bce --load_from rgb --precision 16 --n_frames_extra_val 300 --batch_size_extra_val 2

-------------------------- DeepSpeed Flops Profiler --------------------------
Profile Summary at step 1:
Notations:
data parallel size (dp_size), model parallel size(mp_size),
number of parameters (params), number of multiply-accumulate operations(MACs),
number of floating-point operations (flops), floating-point operations per second (FLOPS),
fwd latency (forward propagation latency), bwd latency (backward propagation latency),
step (weights update latency), iter latency (sum of fwd, bwd and step latency)

params per GPU:                                                         149.62 M
params of model = params per GPU * mp_size:                             0       
fwd MACs per GPU:                                                       12.31 TMACs
fwd flops per GPU:                                                      24.64 T 
fwd flops of model = fwd flops per GPU * mp_size:                       24.64 T 
fwd latency:                                                            1.2 s   
fwd FLOPS per GPU = fwd flops per GPU / fwd latency:                    20.48 TFLOPS

----------------------------- Aggregated Profile per GPU -----------------------------
Top 2 modules in terms of params, MACs or fwd latency at different model depths:
depth 0:
    params      - {'PredictWrapper': '149.62 M'}
    MACs        - {'PredictWrapper': '12.31 TMACs'}
    fwd latency - {'PredictWrapper': '1.2 s'}
depth 1:
    params      - {'EncodePoolClassifyModel': '149.62 M'}
    MACs        - {'EncodePoolClassifyModel': '12.31 TMACs'}
    fwd latency - {'EncodePoolClassifyModel': '1.2 s'}
depth 2:
    params      - {'CLIPBackbone': '149.62 M', 'Identity': '0'}
    MACs        - {'CLIPBackbone': '12.31 TMACs', 'Identity': '0 MACs'}
    fwd latency - {'CLIPBackbone': '1.2 s', 'CosineSimilarityClassifier': '1.15 ms'}
depth 3:
    params      - {'CLIP': '149.62 M', 'VisionTransformer': '86.19 M'}
    MACs        - {'CLIP': '6.17 TMACs', 'VisionTransformer': '6.15 TMACs'}
    fwd latency - {'CLIP': '1.2 s', 'VisionTransformer': '1.11 s'}
depth 4:
    params      - {'Transformer': '122.88 M', 'VisionTransformer': '86.19 M'}
    MACs        - {'VisionTransformer': '6.15 TMACs', 'Transformer': '6.12 TMACs'}
    fwd latency - {'Transformer': '1.18 s', 'VisionTransformer': '1.11 s'}
depth 5:
    params      - {'Sequential': '122.88 M', 'Transformer': '85.05 M'}
    MACs        - {'Sequential': '6.12 TMACs', 'Transformer': '6.11 TMACs'}
    fwd latency - {'Sequential': '1.18 s', 'Transformer': '1.1 s'}
depth 6:
    params      - {'ResidualAttentionBlock': '122.88 M', 'Sequential': '85.05 M'}
    MACs        - {'ResidualAttentionBlock': '6.12 TMACs', 'Sequential': '6.11 TMACs'}
    fwd latency - {'ResidualAttentionBlock': '1.18 s', 'Sequential': '1.1 s'}
depth 7:
    params      - {'ResidualAttentionBlock': '85.05 M', 'Sequential': '81.87 M'}
    MACs        - {'ResidualAttentionBlock': '6.11 TMACs', 'Sequential': '3.92 TMACs'}
    fwd latency - {'ResidualAttentionBlock': '1.1 s', 'Sequential': '662.8 ms'}
depth 8:
    params      - {'Linear': '81.87 M', 'Sequential': '56.67 M'}
    MACs        - {'Linear': '3.92 TMACs', 'Sequential': '3.9 TMACs'}
    fwd latency - {'Sequential': '636.37 ms', 'Linear': '549.82 ms'}
