# Supplementary material for: Streaming Detection of Queried Event Start
Source: arXiv:2412.03567 source file (2024-12-04)
Supplement: Supplementary file 6 [file clip_vainilla_adapter.tex]

python meassure_latency.py --mode predict --task_name sdqes --classification_layer_name cosine_similarity --data_path /vision/u/eatang/sdas/ --video_path /scr/ego4d_full_frames/ --backbone_name qrnn_adapter_clip_ViT-B/16 --eval_freq 5 --epochs 50 --seed 42 --num_workers 16 --gpus 1 --wandb_group vanilla_adapter_60_frames_full --gradient_accumulation_steps 32 --batch_size 4 --n_frames 60 --frame_sample_rate 1 --warmup_epochs 5 --lr 5e-4 --min_lr 5e-6 --wd 0.05 --temporal_pooling_name identity --balance_classes True --criterion_name bce --load_from rgb --precision 16 --balance_classes True --backbone_freeze True --backbone_unfreeze_layer_norm False --adapter_upsample_zero_init True --backbone_qrnn_bidirectional False --backbone_drop_path_rate 0.3 --backbone_proj_after True --num_qrnn_adapters 2 --temporal_pool_backbone False --qrnn_lookback 1 --qrnn_lookahead 0 --adapter_downsample_ratio 0.5 --downsample_qrnn_adapter False --vanilla_adapter True --n_frames_extra_val 300 --batch_size_extra_val 2

-------------------------- DeepSpeed Flops Profiler --------------------------
Profile Summary at step 1:
Notations:
data parallel size (dp_size), model parallel size(mp_size),
number of parameters (params), number of multiply-accumulate operations(MACs),
number of floating-point operations (flops), floating-point operations per second (FLOPS),
fwd latency (forward propagation latency), bwd latency (backward propagation latency),
step (weights update latency), iter latency (sum of fwd, bwd and step latency)

params per GPU:                                                         163.8 M 
params of model = params per GPU * mp_size:                             0       
fwd MACs per GPU:                                                       7.14 TMACs
fwd flops per GPU:                                                      14.29 T 
fwd flops of model = fwd flops per GPU * mp_size:                       14.29 T 
fwd latency:                                                            1.45 s  
fwd FLOPS per GPU = fwd flops per GPU / fwd latency:                    9.86 TFLOPS

----------------------------- Aggregated Profile per GPU -----------------------------
Top 2 modules in terms of params, MACs or fwd latency at different model depths:
depth 0:
    params      - {'PredictWrapper': '163.8 M'}
    MACs        - {'PredictWrapper': '7.14 TMACs'}
    fwd latency - {'PredictWrapper': '1.45 s'}
depth 1:
    params      - {'EncodePoolClassifyModel': '163.8 M'}
    MACs        - {'EncodePoolClassifyModel': '7.14 TMACs'}
    fwd latency - {'EncodePoolClassifyModel': '1.45 s'}
depth 2:
    params      - {'QRNNAdapterCLIPBackbone': '163.8 M', 'Identity': '0'}
    MACs        - {'QRNNAdapterCLIPBackbone': '7.14 TMACs', 'Identity': '0 MACs'}
    fwd latency - {'QRNNAdapterCLIPBackbone': '1.45 s', 'CosineSimilarityClassifier': '1.19 ms'}
depth 3:
    params      - {'VisionTransformer': '100.38 M', 'Transformer': '37.83 M'}
    MACs        - {'VisionTransformer': '7.12 TMACs', 'Transformer': '17.88 GMACs'}
    fwd latency - {'VisionTransformer': '1.36 s', 'Transformer': '81.76 ms'}
depth 4:
    params      - {'Transformer': '99.24 M', 'Sequential': '37.83 M'}
    MACs        - {'Transformer': '7.08 TMACs', 'Conv2d': '40.46 GMACs'}
    fwd latency - {'Transformer': '1.35 s', 'Sequential': '81.48 ms'}
depth 5:
    params      - {'ModuleList': '99.24 M', 'ResidualAttentionBlock': '37.83 M'}
    MACs        - {'ModuleList': '7.08 TMACs', 'ResidualAttentionBlock': '17.88 GMACs'}
    fwd latency - {'ModuleList': '1.34 s', 'ResidualAttentionBlock': '79.6 ms'}
depth 6:
    params      - {'ResidualAttentionBlock': '99.24 M', 'Sequential': '25.2 M'}
    MACs        - {'ResidualAttentionBlock': '7.08 TMACs', 'Sequential': '11.63 GMACs'}
    fwd latency - {'ResidualAttentionBlock': '1.34 s', 'MultiheadAttention': '27.05 ms'}
depth 7:
    params      - {'Sequential': '56.67 M', 'MultiheadAttention': '28.35 M'}
    MACs        - {'Sequential': '3.9 TMACs', 'MultiheadAttention': '2.2 TMACs'}
    fwd latency - {'Sequential': '632.6 ms', 'MultiheadAttention': '389.31 ms'}
