# Supplementary material for: Streaming Detection of Queried Event Start
Source: arXiv:2412.03567 source file (2024-12-04)
Supplement: Supplementary file 10 [file zs_egovlp_clip_4.tex]

python meassure_latency.py --mode predict --task_name sdqes --classification_layer_name cosine_similarity --data_path /vision/u/eatang/sdas/ --video_path /scr/ego4d_full_frames/ --backbone_name egovlp_base --seed 42 --num_workers 16 --wandb_group egovlp_zs --gpus 1 --batch_size 8 --n_frames 60 --frame_sample_rate 1 --temporal_pooling_name identity --criterion_name bce --load_from rgb --precision 16 --backbone_clip_length 4 --n_frames_extra_val 300 --batch_size_extra_val 2

-------------------------- DeepSpeed Flops Profiler --------------------------
Profile Summary at step 1:
Notations:
data parallel size (dp_size), model parallel size(mp_size),
number of parameters (params), number of multiply-accumulate operations(MACs),
number of floating-point operations (flops), floating-point operations per second (FLOPS),
fwd latency (forward propagation latency), bwd latency (backward propagation latency),
step (weights update latency), iter latency (sum of fwd, bwd and step latency)

params per GPU:                                                         180.93 M
params of model = params per GPU * mp_size:                             0       
fwd MACs per GPU:                                                       31.28 TMACs
fwd flops per GPU:                                                      62.61 T 
fwd flops of model = fwd flops per GPU * mp_size:                       62.61 T 
fwd latency:                                                            6.05 s  
fwd FLOPS per GPU = fwd flops per GPU / fwd latency:                    10.35 TFLOPS

----------------------------- Aggregated Profile per GPU -----------------------------
Top 2 modules in terms of params, MACs or fwd latency at different model depths:
depth 0:
    params      - {'PredictWrapper': '180.93 M'}
    MACs        - {'PredictWrapper': '31.28 TMACs'}
    fwd latency - {'PredictWrapper': '6.05 s'}
depth 1:
    params      - {'EncodePoolClassifyModel': '180.93 M'}
    MACs        - {'EncodePoolClassifyModel': '31.28 TMACs'}
    fwd latency - {'EncodePoolClassifyModel': '6.05 s'}
depth 2:
    params      - {'EgoVLPBackbone': '180.93 M', 'Identity': '0'}
    MACs        - {'EgoVLPBackbone': '31.28 TMACs', 'Identity': '0 MACs'}
    fwd latency - {'EgoVLPBackbone': '6.04 s', 'CosineSimilarityClassifier': '1.29 ms'}
depth 3:
    params      - {'FrozenInTime': '180.93 M'}
    MACs        - {'FrozenInTime': '31.28 TMACs'}
    fwd latency - {'FrozenInTime': '6.04 s'}
depth 4:
    params      - {'SpaceTimeTransformer': '114.17 M', 'DistilBertModel': '66.36 M'}
    MACs        - {'SpaceTimeTransformer': '31.28 TMACs', 'DistilBertModel': '5.12 GMACs'}
    fwd latency - {'SpaceTimeTransformer': '5.97 s', 'DistilBertModel': '66.82 ms'}
depth 5:
    params      - {'ModuleList': '113.42 M', 'Transformer': '42.53 M'}
    MACs        - {'ModuleList': '31.11 TMACs', 'VideoPatchEmbed': '161.85 GMACs'}
    fwd latency - {'ModuleList': '5.93 s', 'Transformer': '63.34 ms'}
depth 6:
    params      - {'SpaceTimeBlock': '113.42 M', 'ModuleList': '42.53 M'}
    MACs        - {'SpaceTimeBlock': '31.11 TMACs', 'Conv2d': '161.85 GMACs'}
    fwd latency - {'SpaceTimeBlock': '5.93 s', 'ModuleList': '61.99 ms'}
depth 7:
    params      - {'VarAttention': '56.7 M', 'Mlp': '56.67 M'}
    MACs        - {'VarAttention': '15.56 TMACs', 'Mlp': '15.56 TMACs'}
    fwd latency - {'VarAttention': '3.45 s', 'Mlp': '2.24 s'}
depth 8:
    params      - {'Linear': '113.37 M', 'FFN': '28.33 M'}
    MACs        - {'Linear': '31.11 TMACs', 'FFN': '3.4 GMACs'}
    fwd latency - {'Linear': '4.29 s', 'GELU': '101.53 ms'}
